# Supplementary material for: ATD: Augmenting CP Tensor Decomposition by Self Supervision
Source: arXiv:2106.07900 source file (2022-09-18)
Supplement: Supplementary file 1 [file appendix2.tex]

\section{Reviewer 1}
See reviews in Openreview\footnote{https://openreview.net/forum?id=vs-O9UfzBHQ}.

\medskip
\noindent {\bf Limited novelty}

Section 3.1 more like metric learning but not self-supervised learning since positive pair and negative pair are defined by the latent classes here, not by instance itself. The problem definition is contradictory compared to self-supervised learning.

The self-supervised loss proposed in line\#127 combined positive pairs and negative pairs. From intuitive, which can be a very imbalance, the authors should explain in detail why this can work. Moreover, why popular self-supervised loss (e.g., contrastive-loss) and metric learning loss (e.g., triple-loss) can not be used here? The advantage of loss in line\#127 and the key difference compared to contrastive loss should be highlighted in Section 3.1.

I believe stochastic alternating optimization can not be a novel contribution, since standard CP optimization algorithms (e.g., CP-ALS) can be easily transformed to stochastic version (e.g., stochastic alternating least square (SALS) used in Table 2) via mini-batch updating. I don't see any high-light difference in Algorithm 1.

\medskip
\noindent  {\bf Experiments}

 From Table.1, we can see there are enough labels in training data, so why not constrain the latent distance via labels. The advantage of using self-supervised learning to implement Auxiliary Step is not detailed.

 Why not maintain a fair comparison in Section 4.1, i.e. use the same batch size? And why not compared SALS in Figure 2. The comparison in Section 4.1 seems to be meaningless.

 From Table 2, we can see that two supervised models (i.e., CNN and CNN with Aug) get better performance than tensor models, so how to explain it?

\medskip
\noindent  {\bf Other questions}

 some claims do not have experiments to support, e.g.,
 In the abstract, the authors emphasize that raw tensor data contains redundant information while data augmentation techniques may be used to smooth out noise in samples. The authors should perform controlled noise experiments on raw tensor datasets to support it.

\medskip
\noindent  {\bf  Limitations And Societal Impact}

 Please see the weakness above.
 
 The novelty is limited and experimental comparison seems to be not fair.

 The paper is also kind of overclaim its contributions. This paper only focuses on a very specific type of tensor learning method with CP decomposition. "Augmented Tensor Decomposition" in the title is not proper.

 \section{Reviewer 2}
 
\medskip
\noindent  {\bf  Main Review}

The idea of data augmentation has appeared in CPD and is known as tensorization. The novelty of the proposed method is in deriving the self-supervised loss function and its approximate.

The method which is presented in Section 3.1 for the case supervised learning is related to the discriminant analysis with low-rank CP structure. For unlabelled data, the approximated loss function is also related to the graph regularization method. Both tensor discriminant analysis and graph regularized tensor decomposition are well studied, and should be considered in the simulation.

The proposed loss function computes the distance between the features extracted from the augmented and original data. The derivation of the self-supervised loss is novel, but its efficiency compared to multilinear discriminant analysis and graph regularized CPD is not clear, especially when the approximate function is not much different from the graph regularization term, for example  where  contains normalized row vectors of .

A simple method for augmented CPD is to align the augmented data with the original data to yield a higher order tensor, then apply CPD or graph regularized CPD. For the case studied in the paper, the new data will have order-5, and size . This method has been used e.g., for chromatography–fluorescence excitation–emission data.

The time rotation augmentation method changes the temporal profile of the data and therefore its spectrogram, implying that  and the augmented 
 do not have the same CP decomposition. The first two factor matrices of CPD of  and 
 for spatial and spectral components can be similar, but the last (temporal) factor matrices are different up to certain rotation or permutation.
 
It means that when applying the time rotation, the CP model  and 
 and the loss function  in (9) is incorrect.

\medskip
\noindent  {\bf  Simulations}

In Example 4.1, the authors compared the augmented CPD algorithm (ATD) with a fast algorithm for the ordinary CPD (without any constraint). The results show that ATD improves the classification accuracy 3.8% over Fast CPD. For a more accurate comparison, the authors should compare ATD with graph regularized CPD algorithm or algorithms for CPD or Tucker decomposition for discriminant analysis.

In Example 4.2, the authors compared ATD with SALS, a stochastic algorithm for CPD (and some other methods). Similar to Fast CPD, SALS does not incorporate constraints for better feature extraction.

Table 2 also shows that , i.e., ATD with only the Frobenius norm of the augmented data, and without self-supervised loss, obtains almost similar performance using CPD without augmentation.

There is still question about the benefit of augmented data or the graph regularization term. The authors miss to compare with competitive methods which are directly related, e.g.

CPD of the original data of order-4 (no augmentation) with graph regularization  and Tikhonov regularization

CPD of order-5 augmented data of size  with/without graph regularization term  and Tikhonov regularization

CPD of augmented data of size  with graph regularization term  and Tikhonov regularization, where 
.

\medskip
\noindent  {\bf  Other comments}

A minor error in definition of ,  should be .

"Fast CPD model" -> "Fast CPD algorithm"

"least square" -> "least squares"

Using Nvidea Geforce RTX 3090 GPU at a research institution can be illegal due to EULA https://www.datacenterdynamics.com/en/news/nvidia-updates-geforce-eula-to-prohibit-data-center-use/

\medskip
\noindent  {\bf  Limitations And Societal Impact:}

The paper shows the augmentation method without self-supervised loss does not improve the performance (classification accuracy). This depends on the augmentation method and tensorization method. For example, time rotate changes the factor matrix associated with the temporal profile, i.e., the factor matrix  in the experiment. Therefore, CPDs of the original data and its augmented do not share the same factor matrices as formulated in (9).

The tensorization which aligns data and the augmented data to a tensor of order-5 would work better.

ATD is quite similar to the graph regularized CPD, and graph regularized CPD has been shown to give more discriminant features than the standard CPD.

\section{Reviewer 3}

Overall, the proposed method feels unnatural and a bit contrived. Several key technical points are a bit vaguely described and do not feel correct or convincing.

1. The augmentation method is quite unclear. The paper says “Given a tensor sample $T^{(n)}$, we assume that the augmentation methods, aug() : $T^{(n)}$ $\tilde{T}^{(n)}$, obey the following class-invariance property: $\tilde{T}^{(n)}$ preserves the same class label and admits a component-based representation, specified in Eqn. (1).” This is very hard to parse of follow. How to augment the tensor was not described. More importantly, how to guarantee such class preserving property is perhaps not a trivial question to answer, but the paper did not mention it at all. The footnote “In practice, augmentation methods are chosen based on the input format and application background” feels hand-waving. Note that the entire paper was developed upon this premise. If the augmentation method is not clearly explained and why/how the label preservation can be guaranteed, the latter developments are built upon some blanket promises.

2. I feel very hard to grasp the motivation behind using contrastive learning or SSL where the feature extractor essentially learns a Khatri-Rao (KR) subspace spanned by the Khatri-Rao product of A, B and C. Note that such KR subspace based dimensionality reduction (KR) relies on the shared KR subspace of $T^{(n)}$ and $\tilde{T}^{(n)}$, which this work offered no concrete way to construct, and it has no justification why this is able to learn better embeddings for downstream tasks.

In SSL, the idea is to use powerful feature extractors to extract distortion-invariant information from the original and augmented data. But projectors to KR subspaces are not universal function approximators or feature extractors, and thus are not likely to be as effective as neural networks or kernel functions interns of combatting data distortion.

3. The paper is not easy to read, which could use some re-organization. The section 3.3 “stochastic alternating optimization” is hard to follow. Theorem 2 is supposed to support the convergence in (14), but the equations in Theorem 2 does not look like the update rule in (14). It is also unclear why the fixed point expressed in Theorem 2 is a stationary point of (13). In addition, where is the “stochasticity” of this algorithm. It looks like an incremental algorithm but not stochastic optimization.

4. The novelty of this algorithm seems to be questionable. Using this incremental updates for dynamic tensor decomposition in the presence of streaming data has been quite popular in the signal processing community. For example:

[R1] Nion, D., & Sidiropoulos, N. D. (2009). Adaptive algorithms to track the PARAFAC decomposition of a third-order tensor. IEEE Transactions on Signal Processing, 57(6), 2299-2310.

[R2] Mardani, M., Mateos, G., & Giannakis, G. B. (2015). Subspace learning and imputation for streaming big data matrices and tensors. IEEE Transactions on Signal Processing, 63(10), 2663-2677.

[R3] Shaden Smith, Kejun Huang, Nicholas D Sidiropoulos, and George Karypis. 2018. Streaming Tensor Factorization for Infinite Data Sources. Proceedings of the 2018 SIAM International Conference on Data Mining (SDM’18) (2018).

All these algorithms use a similar structure as the proposed algorithm. The minor difference is that the proposed algorithm deals with 4th order tensor, while [R1]-[R3] dealt with 3rd order tensors. There are also some different regularizations involved in different cases. But the principles are the same.

The technical depth of this work seems to be not deep. The key algorithm does not have any convergence analysis or support. The theorem 1 that connects the population regularizer and the empirical regularizer seems to be straightforward application of concentration theorems. The proof of Theorem 1 is also likely to be wrong. The authors used the Hoeffdings inequality, but did not exhausted all cases over all cases in the considered function class (but only considered a single case). Note that generalization bounds like that in Theorem 1 should be proved by the Hoeffdings inequality (or other concentration theorems) together with some function class complexity measures (e.g., finite class cardinality, VC dimension, and Gaussian/Rademacher complexity). See [R4].
[R4] Shalev-Shwartz, Shai, and Shai Ben-David. Understanding machine learning: From theory to algorithms. Cambridge university press, 2014.
